# Supplementary material for: Rethinking Latent Redundancy in Behavior Cloning: An Information Bottleneck Approach for Robot Manipulation
Source: arXiv:2502.02853 source file (2025-05-13)
Supplement: Supplementary file 2 [file libero_appendix.tex]

\begin{table*}[htbp]
\small
\centering
\caption{Performance on language-condition multi-task benchmark LIBERO. We evaluated 40 tasks of 4 suites using 3 random seeds and reported the average success rate (sr).
The best performance is bolded.
}
\begin{tabular}{
>{\raggedright\arraybackslash}m{3cm}
>{\centering\arraybackslash}m{0.5cm}
>{\centering\arraybackslash}m{2cm}
>{\centering\arraybackslash}m{2.2cm}
>{\centering\arraybackslash}m{2.2cm}
>{\centering\arraybackslash}m{2cm}
>{\centering\arraybackslash}m{1.5cm}
}
\toprule
Method                            &                      & LIBERO-Goal          & LIBERO-Object        & LIBERO-Spatial       & LIBERO-10            & Avg                  \\
\midrule
BC-MLP                            & sr                   & 16.50                & 19.00                & 29.33                & 2.33                 & 16.79                \\
\multirow{1}{*}{BC-MLP+IB}        & sr                   & \textbf{27.67}       & \textbf{31.50}       & \textbf{41.00}       & \textbf{2.67}        & \textbf{25.71}       \\
                                  % & $\beta$                 & 1e-4                 & 1e-4                 & 1e-4                 & 1e-4                 & -                    \\
\midrule
BC-RNN                            & sr                   & 15.17                & 13.33                & 30.67                & 2.33                 & 15.38                \\
\multirow{1}{*}{BC-RNN+IB}        & sr                   & \textbf{26.00}       & \textbf{17.67}       & \textbf{35.17}       & \textbf{3.00}        & \textbf{20.46}       \\
                                  % & $\beta$                 & 5e-3                 & 5e-3                 & 5e-3                 & 5e-3                 & -                    \\
\midrule
BC-Transfomer                     & sr                   & 67.83                & 41.83                & 68.00                & 15.83                & 48.37                \\
\multirow{1}{*}{BC-Transfomer+IB} & sr                   & \textbf{74.17}       & \textbf{45.67}       & \textbf{72.50}       & \textbf{18.00}       & \textbf{52.59}       \\
                                  % & $\beta$                 & 1e-3                 & 1e-4                 & 1e-3                 & 1e-4                 & -                    \\
\midrule
BC-VILT                           & sr                   & 76.17                & 43.00                & 67.17                & 6.50                 & 48.21                \\
\multirow{1}{*}{BC+VILT+IB}       & sr                   & \textbf{83.83}       & \textbf{52.00}       & \textbf{70.67}       & \textbf{8.67}        & \textbf{53.79}       \\
                                  % & $\beta$                 & 5e-3                 & 5e-3                 & 1e-3                 & 1e-4                 & -                     \\
\bottomrule
\end{tabular}
\label{tab:libero_appendix}
\end{table*}
